# Supplementary material for: On RAC Drawings of Graphs with one Bend per Edge
Source: arXiv:1808.10470 source file (2018-08-30)
Supplement: Supplementary file 1 [file appendix.tex]

%=================================================================
\section*{\LARGE Appendix}
%=================================================================
